# Supplementary material for: A Multivariate Multilevel Longitudinal Functional Model for Repeatedly Observed Human Movement Data
Source: arXiv:2408.08481 source file (2024-08-16)
Supplement: Supplementary file 1 [file simulation-limitations.tex]

\section{Simulation Limitations}

\begin{itemize}
    \item Shapes of functions restricted to quadratic
    \item Mean number of strides should be a random variable.
    \item Low rank (i.e., $K=10$)
    \item Skewed missingness!
    \item Two covariates!
    \item Signal to noise ratio
    \item Discontinuities.
    \item Heavy-tailed error
\end{itemize}
